# Supplementary material for: Knowledge Graph-Enhanced Zero-Shot Topic Classification: A Multi-Strategy Comparative Study
Source: arXiv:2605.30465 source file (2026-08-07)
Supplement: Supplementary file 1 [file appendix.tex]

\section{Appendix}

% \subsection{DSPy Signatures}

% \subsubsection{Graph Construction Signatures}

% \paragraph{Stage 1: Entity Extraction.}
 
% \begin{tcolorbox}[enhanced,breakable,colback=gray!8,colframe=gray!40,
%   boxrule=0.4pt,arc=2pt,left=4pt,right=4pt,top=3pt,bottom=3pt]
% \begin{lstlisting}[style=sigstyle]
% class EntityExtractor(dspy.Signature):
%     """Extract key entities from the given text. Extracted entities are nouns, verbs, or adjectives, particularly regarding sentiment. This is for an extraction task, please be thorough and accurate to the reference text.
 
%     Return ONLY a valid JSON list format:
%     ["entity1", "entity2", "entity3"]"""
%     text = dspy.InputField(desc="The text to extract entities from")
%     entities = dspy.OutputField(desc="List of extracted entities in JSON format")\end{lstlisting}
% \end{tcolorbox}
 
% \paragraph{Stage 2 --- Relation Extraction.}
 
% \begin{tcolorbox}[enhanced,breakable,colback=gray!8,colframe=gray!40,
%   boxrule=0.4pt,arc=2pt,left=4pt,right=4pt,top=3pt,bottom=3pt]
% \begin{lstlisting}[style=sigstyle]
% class RelationExtractor(dspy.Signature):
%     """Extract subject-predicate-object triples from the assistant message. A predicate (1-3 words) defines the relationship between subject and object. Subject and object are entities from the provided list. This is an extraction task; be thorough, accurate, and faithful to the reference text.
 
%     Return ONLY valid JSON format:
%     [["subj1","pred1","obj1"],["subj2","pred2","obj2"]]"""
%     text = dspy.InputField(desc="The text to extract relations from")
%     entities = dspy.InputField(desc="List of available entities")
%     triples  = dspy.OutputField(desc="List of [subject, predicate, object] "
% "triples in JSON format")
% \end{lstlisting}
% \end{tcolorbox}
 
% \paragraph{Stage 3 --- Cluster Validation.}
 
% After relation extraction, \texttt{all-MiniLM-L6-v2} groups entities by cosine similarity (threshold 0.75). Candidate clusters of 2--4 entities are validated by the following signature before merging.

\subsubsection{Classification Signatures}
\label{app:signatures:classification}

The knowledge graph is serialized into the following format before being passed to any classification signature. If the graph has no edges, the field reads \texttt{"No knowledge graph available."}
 
\begin{tcolorbox}[enhanced,colback=gray!8,colframe=gray!40,
  boxrule=0.4pt,arc=2pt,left=4pt,right=4pt,top=3pt,bottom=3pt]
\begin{lstlisting}[style=sigstyle]
Knowledge Graph:
Entities: entity1, entity2, entity3, ...
 
Relationships:
entity1 --[predicate]--> entity2
entity2 --[predicate]--> entity3
...                       
\end{lstlisting}
\end{tcolorbox}
 
\paragraph{Variant A --- Article Graph Classification (AG)}

\paragraph{Variant B --- Keyword-Enhanced Classification (AKG)}
 
Topics are passed as one entry per line, e.g.\
\texttt{Mental Health (keywords: depression, anxiety, ...)},
with up to 10 keywords per topic.

\paragraph{Variant C --- AG + Self-Consistency (AGS)}
 
Called $N{=}5$ times at temperature $0.5$. A topic is retained only if it appears in at least 2 of the 5 runs.

\paragraph{Variant D --- AKG + Self-Consistency (AKGS)}
 
Same majority-vote aggregation as Variant~C ($N{=}5$, temperature $0.5$).
 
\begin{tcolorbox}[enhanced,breakable,colback=gray!8,colframe=gray!40,
  boxrule=0.4pt,arc=2pt,left=4pt,right=4pt,top=3pt,bottom=3pt]
\begin{lstlisting}[style=sigstyle]
class ConsensusClassificationWithKeywords(dspy.Signature):
    """Classify topics using provided keywords as guidance. Keywords help understand what each topic represents. Match article content and KG against keywords. Be precise; return 1-3 topics CLEARLY discussed. If uncertain, be conservative."""
    article_text : str = dspy.InputField(desc="Article content")
    kg_summary : str = dspy.InputField(desc="Knowledge graph summary")
    available_topics_with_keywords: str = dspy.InputField(desc="Topics with keywords: "
             "'topic (keywords: kw1, kw2, ...)'")
    predicted_topics: str = dspy.OutputField(desc="1-3 relevant topics or 'none'. "
"ONLY names from available_topics.")
\end{lstlisting}
\end{tcolorbox}
